# Supplementary material for: Data-driven Optimization for the Evolve-Filter-Relax regularization of convection-dominated flows
Source: arXiv:2501.03933 source file (2025-04-12)
Supplement: Supplementary file 1 [file appendix_old.tex]

\subsection{CASE 1: $Re_{max}=100$}
\label{re-100}

In this Section, we consider a comparison among the results from the following full-order simulations:

\begin{itemize}
    \item[1.] Direct Navier--Stokes (DNS) with the refined mesh \subref{mesh-ref};
    \item[2.] Evolve--Filter--Relax (EFR) with the coarse mesh \subref{mesh-coarse}, for different $\delta$ values, with fixed $\chi=5\Delta t$, where $\Delta t=\SI{4e-4}{\second}$ is the time step used in simulations;
    \item[3.] Evolve--Filter--Relax (EFR) with the coarse mesh \subref{mesh-coarse}, with fixed $\delta=0.0032$, for different $\chi$ values.
\end{itemize}

On the other hand, Figure \ref{fig:norms-varying-chi-re100} displays the norms of the velocity and pressure fields.
In these plots, the norms of the fields resulting from the simulations with the coarse mesh are very similar to those obtained from the high-fidelity simulation.

\medskip

Figure \ref{fig:errs-varying-chi-re100} represents the velocity and pressure errors \eqref{eq:errs-full-coarse} with respect to the high-fidelity fields evaluated on the refined mesh. From Figure \ref{fig:errs-varying-chi-re100}, we can notice that the accuracy of the fields improves as $\chi$ tends towards $0$, i.e., as the contribution of the filtered solution in the EFR system decreases until vanishing.
Thus, we can conclude that the EFR regularization does not improve the results of the DNS simulation in this specific test case. The reason for this is that for small $Re$ the DNS already provides accurate results, even when a course mesh is used.

We here report the maximum value for the lift coefficient for different $\chi$, in order to make a comparison with the result obtained from the reference DNS simulation on the finest mesh.
\begin{itemize}
    \item DNS on mesh refined: $C_{l, max}=0.456$;
    \item DNS on mesh coarse: $C_{l, max}=0.450$;
    \item EFR ($\delta=0.0032$, $\chi=dt$): $C_{l, max}=0.421$;
    \item EFR ($\delta=0.0032$, $\chi=2dt$): $C_{l, max}=0.399$;
    \item EFR ($\delta=0.0032$, $\chi=3dt$): $C_{l, max}=0.376$;
    \item EFR ($\delta=0.0032$, $\chi=4dt$): $C_{l, max}=0.351$;
    \item EFR ($\delta=0.0032$, $\chi=5dt$): $C_{l, max}=0.326$.
\end{itemize}
It is evident that the EFR is not successful for this test case.

\begin{figure}[h!]
    \centering
    \includegraphics[width=0.9\textwidth]{images/norms_delta_0032_varying_chi_paper.pdf}
    \caption{Norms of full-order solutions of EFR simulations (at $Re_{max}=100$) for different $\chi$ values, with $\delta=0.0032$, considering the coarse mesh and the refined one.}
    \label{fig:norms-varying-chi-re100}
\end{figure}

\begin{figure}[h!]
    \centering
    \includegraphics[width=0.9\textwidth]{images/err_delta_0032_varying_chi_paper.pdf}
    \caption{Relative errors of full-order solutions of EFR simulations (at $Re_{max}=100$) for different $\chi$ values, with $\delta=0.0032$.}
    \label{fig:errs-varying-chi-re100}
\end{figure}
In the following Subsections, we will try to consider higher Reynolds numbers, for which the standard Navier--Stokes formulation fails in simulating the flow.

\begin{figure}
    \centering    \subfloat{\includegraphics[width=0.9\textwidth, trim={0cm 1.5cm 0cm 1.5cm}, clip]{images/time_8_DNS_ref.png}}\\
    \subfloat{\includegraphics[width=0.9\textwidth, trim={0cm 1.5cm 0cm 1.5cm}, clip]{images/time_8_DNS_coarse.png}}\\
    \subfloat{\includegraphics[width=0.9\textwidth, trim={0cm 3cm 0cm 3cm}, clip]{images/time_8_FOMs_chi_00032.png}}
    \caption{Velocity and pressure fields at  the final time step $t=8$ for DNS and EFR simulations, at $Re_{max}=100$.}
    \label{fig:plots_re100}
\end{figure}
\newpage

\subsection{CASE 2: $Re_{max}=300$}
\label{re-300}

\begin{figure}[h!]
    \centering
    \includegraphics[width=0.9\textwidth]{images/norms_varying_delta_Re300.pdf}
    \caption{Norms of full-order solutions of EFR simulations (at $Re_{max}=300$) for different $\delta$ values, with $\chi=5 \Delta t$, considering all the different meshes.}
    \label{fig:norms-varying-chi-re300}
\end{figure}

\begin{figure}[h!]
    \centering
    \includegraphics[width=0.9\textwidth]{images/errs_varying_delta_Re300.pdf}
    \caption{Relative errors of full-order solutions of EFR simulations (at $Re_{max}=300$) for different $\delta$ values, with $\chi=5 \Delta t$.}
    \label{fig:errs-varying-delta-re300}
\end{figure}

At $Re_{max}=300$ we can still notice that the results obtained with a standard Navier--Stokes simulation outperform the EFR results even on a coarse mesh, as can be seen from Figures \ref{fig:errs-varying-delta-re300} and \ref{fig:norms-varying-chi-re300}.

We here report the maximum value for the lift coefficient for different $\delta$ and for DNS simulations con coarse, medium and fine mesh.
\begin{itemize}
    \item DNS on mesh refined: $C_{l, max}=2.63$;
    \item DNS on mesh medium: $C_{l, max}=2.54$;
    \item DNS on mesh coarse: $C_{l, max}=2.35$;
    \item EFR ($\delta=0.0032$, $\chi=5\Delta t$): $C_{l, max}=1.98$;
    \item EFR ($\delta=0.0032$, $\chi=2\Delta t$): $C_{l, max}=0.99$.
\end{itemize}

\begin{figure}
    \centering    \subfloat{\includegraphics[width=0.9\textwidth, trim={0cm 1cm 0cm 1cm}, clip]{images/time_8_DNS_ref_Re300.png}}\\
    \subfloat{\includegraphics[width=0.9\textwidth, trim={0cm 1cm 0cm 1cm}, clip]{images/time_8_DNS_med_Re300.png}}\\
    \subfloat{\includegraphics[width=0.9\textwidth, trim={0cm 1cm 0cm 1cm}, clip]{images/time_8_DNS_coarse_Re300.png}}\\
    \subfloat{\includegraphics[width=0.9\textwidth, trim={0cm 2cm 0cm 2cm}, clip]{images/plots_delta.png}}
    \caption{Velocity and pressure fields at  the final time step $t=8$ for DNS and EFR simulations (at constant $\chi=5\Delta t$), at $Re_{max}=300$.}
    \label{fig:plots_re300}
\end{figure}

The following Subsection will focus on a higher value of the Reynolds number, where the classic DNS formulation fails before the end time of the simulation.

% Part with sensitivity study on Re_max=350 WITHOUT machine learning staff
\begin{comment}
For this reason, the EFR formulation can be suitable for this test case.
In Figure \ref{fig:fields_DNS_re350} the velocity and pressure fields of no-EFR simulations are displayed at the final time instant $t=8$ s. In Figures \ref{fig:fields_EFR_deltalow}, \ref{fig:fields_EFR_deltalow2} and \ref{fig:fields_EFR_deltahigh} we show the fields for different values of $\delta$ and $\chi$.

More in detail, when the value of $\delta$ is smaller ($\delta=0.0032$) the residual of the EFR system significantly increases in the last time steps, leading to the generation of spurious oscillation nearby the outlet of our domain, as shown in Figure \ref{fig:fields_EFR_deltalow}.

Increasing the value of $\delta$ to $0.00525$ and for $\chi=5\Delta t$ (Figure \ref{fig:fields_EFR_deltalow2}), the simulation does not explode anymore. However, the plots of the errors and norms in Figure \ref{fig:errors_chi_re350} show that $\delta=0.00525$ is unstable for low values of $\chi$, i.e. decreasing the filtering contribution in the \emph{relax} step.

From Figures \ref{fig:errs_deltahigh_chilow_re350} and \ref{fig:norms_deltahigh_chilow_re350}, we notice that increasing the value of $\delta$ for low $\chi=\Delta t$, the simulations reach convergence at each time step, but the resulting fields are more diffusive, reaching poorer results in terms of accuracy with respect to our reference fields.

\begin{figure}[h!]
    \centering
    \subfloat[Fields at time $t=8$ (on refined mesh)]{\includegraphics[width=0.9\textwidth, trim={0cm 2cm 0cm 2cm}, clip]{images/time_8_DNS_ref_Re350.png}}\\
    \subfloat[Fields at time $t=8$ (on medium mesh)]{\includegraphics[width=0.9\textwidth, trim={0cm 2cm 0cm 2cm}, clip]{images/time_8_DNS_med_Re350.png}}
    \caption{Representations of the velocity and pressure fields for DNS simulations on refined and medium meshes, at $Re_{max}=350$.}
    \label{fig:fields_DNS_re350}
\end{figure}

\begin{figure}[h!]
    \centering
    \includegraphics[width=0.9\textwidth]{images/plots_chi_time_8_delta_0032.png}
    \caption{Representations of the velocity and pressure fields for EFR simulations for $\delta=0.0032$, at time $t=8$ and $Re_{max}=350$.}
    \label{fig:fields_EFR_deltalow}
\end{figure}
 
\begin{figure}[h!]
    \centering
    \includegraphics[width=0.9\textwidth]{images/plots_chi_time_8_delta_00525.png}
    \caption{Representations of the velocity and pressure fields for EFR simulations for $\delta=0.00525$, at time $t=8$ and $Re_{max}=350$.}
    \label{fig:fields_EFR_deltalow2}
\end{figure}

\begin{figure}[h!]
    \centering
    \includegraphics[width=0.9\textwidth]{images/plots_highdeltas_chidt_time_8.png}
    \caption{Representations of the velocity and pressure fields for EFR simulations for different $\delta$ values, at time $t=8$ and $Re_{max}=350$.}
    \label{fig:fields_EFR_deltahigh}
\end{figure}

\begin{figure}[h!]
    \centering    
    \subfloat{\includegraphics[width=0.9\textwidth]{images/lift_delta0032.png}}\\
    \subfloat{\includegraphics[width=0.9\textwidth]{images/lift_delta00525.png}}\\
    \subfloat{\includegraphics[width=0.9\textwidth]{images/lift_delta0073.png}}
    \caption{Lift coefficients for EFR simulations at different $\delta$ values, at $Re_{max}=350$. Results are compared with the DNS simulations.}
    \label{fig:lifts_re350}
\end{figure}

\begin{figure}[h!]
    \centering    
    \subfloat[$\delta=0.0032$]{\includegraphics[width=0.9\textwidth]{images/errs_varying_chi_delta0032_Re350.png}}\\
    \subfloat[$\delta=0.00525$]{\includegraphics[width=0.9\textwidth]{images/errs_varying_chi_delta00525_Re350.png}}\\
    \subfloat[$\delta=0.0073$]{\includegraphics[width=0.9\textwidth]{images/errs_varying_chi_delta0073_Re350.png}}
    \caption{Errors for EFR simulations at different $\delta$ and $\chi$ values, at $Re_{max}=350$. Results are compared with the DNS simulations.}
    \label{fig:errors_chi_re350}
\end{figure}

\begin{figure}[h!]
    \centering 
    \includegraphics[width=0.9\textwidth]{images/errs_varying_delta_Re350.png}
    \caption{Errors for EFR simulations at different $\delta$ values with $\chi=5\Delta t$ fixed, at $Re_{max}=350$. Results are compared with the DNS simulations.}
    \label{fig:errors_delta_re350}
\end{figure}

\begin{figure}[h!]
    \centering 
    \includegraphics[width=0.9\textwidth]{images/norms_varying_delta_Re350.png}
    \caption{Norms for EFR simulations at different $\delta$ values with $\chi=5\Delta t$ fixed, at $Re_{max}=350$. Results are compared with the DNS simulations.}
    \label{fig:norms_delta_re350}
\end{figure}

\begin{figure}[h!]
    \centering 
    \includegraphics[width=0.9\textwidth]{images/errs_varying_delta_chi1dt_Re350.png}
    \caption{Relative errors for EFR simulations, with respect to the DNS simulation on refined mesh, at different $\delta$ values with $\chi=\Delta t$ fixed, at $Re_{max}=350$.}
    \label{fig:errs_deltahigh_chilow_re350}
\end{figure}

\begin{figure}[h!]
    \centering 
    \subfloat[Norms]{\includegraphics[width=0.9\textwidth]{images/norms_varying_delta_chi1dt_Re350.png}}\\
    \subfloat[Zoom on plots]{\includegraphics[width=0.9\textwidth]{images/norms_zoom_varying_delta_chi1dt_Re350.png}}
    \caption{Norms for EFR simulations at different $\delta$ values with $\chi=\Delta t$ fixed, at $Re_{max}=350$. Results are compared with the DNS simulations.}
    \label{fig:norms_deltahigh_chilow_re350}
\end{figure}
\end{comment}
